# Supplementary material for: A fast solver for the spatially homogeneous electron Boltzmann equation
Source: arXiv:2409.00207 source file (2024-08-30)
Supplement: Supplementary file 1 [file appendix.tex]

\section{Matching particle and PDE methodology}

\subsection{Cross Sections}

The scattering differential cross section is given by
\begin{equation}
    \sigma(\theta) = \frac{b}{\sin{\theta}} \bigg| \frac{db}{d \theta} \bigg|
\end{equation}
Now we need to figure out $b$, which by some trig and geometry stuff is given by

\begin{equation}
    b = \frac{qQ}{2E} \cot{(\frac{\theta}{2})}
\end{equation}
Here, $E = \frac{1}{2}mv^2$, which we will substitute later. For now, this leads us to

\begin{equation}
    \frac{db}{d\theta} = \frac{qQ}{2E} \frac{-1}{2\sin^2{(\frac{\theta}{2})}}
\end{equation}
Now we want to put this back into our original equation. Putting this all together, we get

\begin{equation}
    \sigma(\theta) = (\frac{b}{\sin(\theta)}) (\frac{qQ}{2E})(\frac{1}{\sin^2(\frac{\theta}{2})}
\end{equation}
We now note that $2E = mu^2$ and that $m = 2m_{ab}$. Simplifying this down (I checked the math out here), we get

\begin{equation}
    \sigma(\theta) = \frac{q^4}{4m_{ab}^2 u^4 \sin^4(\frac{\theta}{2})}
\end{equation}
which matches the Rosenbluth paper as desired.

\subsection{Change of reference frame}

If we consider our relative velocity vector $u = (u_x, u_y, u_z) = \sum_{j=1}^3 u_j e_j$, where $e_j$ are the traditional Cartesian unit vectors, then we define a new coordinate system $e_1', e_2', e_3'$ such that

\begin{equation}
    e_1' = \frac{u}{\big| u \big|}
\end{equation}
\begin{equation}
    e_2' = \frac{e_3 \times u}{(u_x^2 + u_y^2)^{\frac{1}{2}}}
\end{equation}
\begin{equation}
    e_3' = e_1' \times e_2'
\end{equation}
We now consider the relative velocity to have components $u_L^j$ in this reference frame. In fact, $u_L = (\big|u\big|, 0, 0)$ initially in this prime reference frame. We now have $u_L$ going through a rotation by an angle $\theta$ about the $e_3'$ axis and by an angle $\phi$ about the $e_1'$ axis. This gives us rotation matrices

$R_{\theta} = \begin{pmatrix}
    \cos(\theta) & -\sin(\theta) & 0\\
    \sin(\theta) & \cos(\theta)  & 0\\
    0              & 0               & 1
\end{pmatrix}, 
R_{\phi} = \begin{pmatrix}
    1 & 0 & 0\\
    0 & \cos(\phi) & -\sin(\phi)\\
    0 & \sin(\phi) & \cos(\phi)
\end{pmatrix}
$ 
We now compute $\Delta u_L = R_{\phi} R_{\theta} u_L - u_L$ and find that
\begin{equation}
\begin{split}
    \Delta u_l^1 = \big|u\big|(\cos(\theta)-1) \\
    \Delta u_l^2 = \big|u\big| \cos(\phi)\sin(\theta) \\
    \Delta u_l^3 = \big|u\big| \sin(\phi)\sin(\theta)
\end{split}
\end{equation}
This can be transformed using trig identities to get 
\begin{equation}
\begin{split}
    \Delta u_l^1 = -2\big|u\big| \sin^2(\frac{\theta}{2})\\
    \Delta u_l^2 = 2\big|u\big|  \sin(\frac{\theta}{2})\cos(\frac{\theta}{2})\cos(\phi)\\
    \Delta u_l^3 = 2\big|u\big| \sin(\frac{\theta}{2}) \cos(\frac{\theta}{2}) \sin(\phi)
\end{split}
\end{equation}
From here, we can convert back to solve for $\Delta_u^{\mu}$, the change in the components of $u$ in the fixed coordinate system, for each coordinate direction $\mu=x,y,z$. Product terms can be simply gotten by multiplying two terms for different values $\mu, \mu'$. This is given by
\begin{equation}
    \Delta u^{\mu} = (e_{\mu} \cdot e_{\nu}') \Delta u_L^{\nu}
\end{equation}
Note that these are exact values and not integrated over any angles, but rather are a function of the angles $\theta, \phi$. Using Mathematica, we find these values to be 
\begin{equation}
    \begin{split}
        \Delta u^x = \frac{u_x u_z \sin(\theta)\cos(\phi)}{u_p} -\frac{u_y \big|u\big| \sin(\theta) \sin(\phi)}{u_p} - u_x(1-\cos(\theta)) \\
        \Delta u^y = \frac{u_y u_z \sin(\theta)\cos(\phi)}{u_p} +\frac{u_x \big|u\big| \sin(\theta) \sin(\phi)}{u_p}- u_y(1-\cos(\theta)) \\
        \Delta u^z = -u_p \sin(\theta) \cos(\phi) - u_z(1-\cos(\theta))
    \end{split}
\end{equation}
We note that these expressions differ from the standard formula presented originally by the Takizuka and Abe. That is, these papers report 
\begin{equation}
    \begin{split}
        \Delta u^x = -\frac{u_x u_z \sin(\theta)\sin(\phi)}{u_p} -\frac{u_y \big|u\big| \sin(\theta) \cos(\phi)}{u_p} - u_x(1-\cos(\theta)) \\
        \Delta u^y = -\frac{u_y u_z \sin(\theta)\sin(\phi)}{u_p} +\frac{u_x \big|u\big| \sin(\theta) \cos(\phi)}{u_p}- u_y(1-\cos(\theta)) \\
        \Delta u^z = u_p \sin(\theta) \sin(\phi) - u_z(1-\cos(\theta))
    \end{split}
\end{equation}
While the expressions differ, we note that the two formulas, which use different treatments regarding $\phi$, prove to give identical results using our particle code.

\subsection{Integrated over for PDE}
We now want to look at the change of relative velocity for all collisions by integrating over the scattering angles $\theta, \phi$ (which in the below equation is shown together as $d\Omega$. We know that this term looks like 
\begin{equation}
    \{ \Delta u_L^{\mu} \} = \int d\Omega \sigma(\theta,\big|u\big|) \big|u\big| (\Delta u_L^{\mu})
\end{equation}

We now consider just the first direction ($\mu= 1$). We note that there is no $\phi$ dependence, meaning our Jacobian setup can be simplified as $\int_0^{\pi} \int_0^{2\pi} \sin(\theta) d\phi d\theta = 2\pi \int_0^{\pi} \sin(\theta) d\theta$. We can then write (I verified this is correct)
\begin{equation}
    \{ \Delta u_L^1 \} = \bigg(\frac{-\pi e^4}{m_{ab}^2 \big|u\big|^2}\bigg)\int_0^{\pi} \frac{\sin(\theta)}{\sin^2(\frac{\theta}{2})} d\theta
\end{equation}

This integral diverges logarithmically at small angles, so a cutoff at $\theta_{\mathrm{min}}$ is introduced. The integral part becomes $4\log(\sin(\frac{2}{\theta_{\mathrm{min}}}))$. For small values of $x$, $\sin{x} \approx x$, so we can simplify and approximate as

\begin{equation}
    \Delta u_L^1 = \big( \frac{-4 \pi e^4}{m_{ab}^2 u^2} \big) \log{XXX} \frac{2}{\theta_{\mathrm{min}}}
\end{equation}

Now something happens, and we write $\log(\frac{2}{\theta_{\mathrm{min}}}) = \log(D)$, where

\begin{equation}
    \begin{split}
        & D = \frac{1}{2}m_{ab} u^2 (\frac{\lambda_D}{e^2}) \\
        & \lambda_D = \bigg( \frac{kT}{4\pi n_e e^2} \bigg) ^{\frac{1}{2}}
    \end{split}
\end{equation}

We can use the substitution

% web.uvic.ca/~rdesousa/tea1ng/P321A/L20_321A.pdf

\subsection{Rosenbluth and Landau equality}
The Landau equation can be written as 
\begin{equation}
    \begin{split}
        \frac{\partial f}{\partial t} = \frac{\partial}{\partial v_i} = \int K_{ij} \bigg(f' \frac{\partial f}{\partial v_j} - f \frac{\partial f'}{\partial v_j'}\bigg) d\mathbf{v'} \\
        K_{ij} = K_d \frac{\omega^2 \delta_{ij} - \omega_i \omega_j}{\omega^3}
    \end{split}
\end{equation}

Here we have $f = f(\mathbf{v},t)$, $f' = f(\mathbf{v}',t)$, and $w = v - v'$ to be the relative velocity. We first want to rewrite this equation in the Fokker-Planck form. Recall that a multidimensional Fokker-Planck equation takes the form of 

\begin{equation}
    \frac{\partial p(\mathbf{x},t)}{\partial t} = \frac{\partial}{\partial x_i} \big[\mu_i(\mathbf{x},t)p(\mathbf{x},t)\big] + \frac{\partial^2}{\partial x_i \partial x_j} \big[D_{ij}(\mathbf{x},t)p(\mathbf{x},t)\big]
\end{equation}

\section{DSMC Method}
\subsection{DSMC Stepping}
Restrictions on timestep: we measure error as missed collisions in a timestep for a given particle. We want this error $r$ to be $r < 0.01$, which requires $P_i < 0.095$. This gives the timestep set to be such that $\Delta t \leq \frac{0.1}{\nu_i \|\|v_i\|\|}$ for all possible particles. We estimate the max of $\|\|v_i\|\| = $ and max of other things to be such and such. 

\subsection{Null Collision Method}
Much of the literature regarding PIC and DSMC codes use the null collision method. In this method, a maximum collision probability, $P_{\mathrm{NULL}}$, is precomputed at the beginning of the simulation. At each timestep, a random subset of the particles of size $P_{\mathrm{NULL}} N$ is considered for collision, and the remaining particles will not collide . Because $P_{\mathrm{NULL}}$ is typical on the order of $10^{-2}$, this in essence reduces the problem size greatly. We find, however, that for our code this code is ultimately not a speedup and is in fact slower due to this selection process. The computation required for collisions is negligible compared to the cost of selecting the particle subset for collisions.

\section{DSMC: Calculating $l$-modes}

We use spherical harmonics to approximate the probability density function $f(v_r, v_\theta)$ as 

\begin{equation}
f(v_r, v_\theta) = \sum_{l=0}^{l'} f_l(v_r) Y_{l0}(v_\theta)
\end{equation}

Note that this includes the assumption of uniformity in $\phi$ as well as only considers the 0 spherical harmonic in something. 

The PDE code solves directly for $f_l$. The PIC code models particles, so these functions are calculated in a post-processing step. Due to orthogonality of the $f_l$, they can be calculated using an inner product, giving us

\begin{equation}
f_l(v_r) = 2 \pi \int_0^{2\pi} f(v_r, v_{\theta}) Y_{l0} \sin(v_{\theta}) d\theta
\end{equation}

\begin{equation}
f_l(v_r^j) = \frac{2\pi}{N} \sum_{i=1} f(v_r^j, v_\theta^i)
\end{equation}

Particles are binned according to their energy $v_r$. For each energy bin $v_r^j$, Monte Carlo integration is used to determine the value of $f_l(v_r^j)$. This given by

\begin{equation}
f_l(v_r^j) = \frac{1}{N} \sum_j^{N_i} Y_{l0}(v_\theta^i)
\end{equation}

We then determine a normalization constant $M$, where

\begin{equation}
    M = \int_0^\infty f_0(v_r) \sqrt{v_r} dv_r
\end{equation}

and then normalize each $f_l$ as $f_l = \frac{f_l}{M}$.

\section{For TST}

\begin{table}[H]
\centering
\begin{tabular}{|c|c|c|c|c|c|c|}
    \hline
     &  $10^{-1}$ & $10^{-2}$ & $10^{-3}$ & $10^{-4}$ & $10^{-5}$ & $10^{-6}$ \\
    \hline
    \hline
    Mean energy & $2.1\times 10^{-3}$ & $1.5\times 10^{-3}$ & $6.9\times 10^{-4}$ & $1.6\times 10^{-3}$ & $8.9\times 10^{-4}$ & $3.1\times 10^{-4}$ \\
    \hline
    Elastic rate coefficient & $3.3\times 10^{-3}$ & $5.4\times 10^{-3}$ & $8.2\times 10^{-3}$ & $9.8\times 10^{-3}$ & $9.8 \times 10^{-3}$ & $8.3 \times 10^{-3}$ \\
    \hline
    Ionization rate coefficient & $1.1\times 10^{-2}$ & $5.7\times 10^{-3}$ & $1.1\times 10^{-2}$ & $7.3\times 10^{-3}$ & $9.1\times 10^{-4}$ & $4.8\times 10^{-4}$ \\
    \hline
    Electron mobility & $2.5\times 10^{-3}$ & $1.3\times 10^{-3}$ & $5.9\times 10^{-3}$ & $4.1\times 10^{-3}$ & $3.5\times 10^{-3}$ & $3.2\times 10^{-3}$ \\
    \hline
\end{tabular}
\caption*{Relative errors between particle code and Bolsig. $\frac{E}{N} = 20\mathrm{Td}$. $n_0 = 3.22 \times 10^{22} \frac{1}{m^3}$}
\end{table}

\begin{equation}
    \begin{split}
    \delta \equiv \tan{(\frac{\theta}{2})} \\
    \langle \delta^2 \rangle = \frac{q_e^4 n_e \Delta t \log{\Lambda}}{2 \pi \epsilon_0^2 m_e^2 u^3} \\
    \phi \in \big[0, 2\pi\big]
    \end{split}
\end{equation}

\begin{table}[H]
\centering
\begin{tabular}{|c|c|c|}
    \hline
     N & Tioga time (ms) & Lassen time (ms) \\
    \hline
    \hline
    $50,000$ & $2.1$ & $0.18$\\
    \hline
    $100,000$ & $4.7$ & $1.01$\\
    \hline
    $200,000$ & $9.89$ & $3.43$\\
    \hline
    $400,000$ & $20.2$ & $8.27$\\
    \hline
    $800,000$ & $40.9$ & $18.0$\\
    \hline
    $1,600,000$ & $82.4$ & $37.5$\\
    \hline
    $3,200,000$ & $165.4$ & $76.6$\\
    \hline
\end{tabular}
\caption*{Wall clock time per step: electron kernel}
\end{table}

$\frac{E}{N} = 20\mathrm{Td}$. Ionization fraction = $10^{-4}$. $n_0 = 3.22 \times 10^{22} \frac{\#}{m^3}$
